# Supplementary material for: Quantitative Understanding of VAE as a Non-linearly Scaled Isometric Embedding
Source: arXiv:2007.15190 source file (2023-02-22)
Supplement: Supplementary file 1 [file Appendix.tex]

\if0
%%%%%%%%%%%%%%%%%%%%%%%%%%%%%%%%%%%%%%%%%%%%%%%%%%%%%%%%%%%%%%%%
\section{Approximation of reconstruction loss as quadratic form}
\subsection{Approximation of distortion in uniform quantization}
\label{sec:ApproxRDTheory}
 Let $T$ be a quantization step.  Quantized values $\hat {z_{j}}$ is derived as $k \ T$, where $k = \mathrm{round}( {z_j} / T)$. 
Then $d$, the distortion per channel, is approximated by 
\begin{eqnarray}
\label{EQ_Noise}
%d \simeq \int_{\hat {z_{j}}-T/2}^{\hat {z_{j}}+T/2} (z_j-\hat {z_{j}})^2 \cdot \frac{1}{T} \ \mathrm{d} z_j = \frac{T^2}{12}
d 
&=& \sum_{k}\int_{(k+1/2)T}^{(k-1/2)T} p(z_j)(z_j-k\ T)^2 \ \mathrm{d} z_j  \nonumber \\
&\simeq& \sum_{k}p(k \ T)\int_{(k+1/2)T}^{(k-1/2)T} (z_j-k\ T)^2  \ \mathrm{d} z_j  \nonumber \\ 
&=& \frac{T^3}{12}\sum_{k}p(k \ T)  \nonumber \\ 
&\simeq& \frac{T^2}{12}.
\end{eqnarray}
Here, $\sum_{k}T\ p(k \ T) \simeq 1$ is used.
%
%%%%%%%%%%%%%%%%%%%%%%%%%%%%%%%%%%%%%%%%%%%%%%%%%%%%%%%%%%%%%%%%
\subsection{Approximation of reconstruction loss}
\label{sec:ApproxRecLoss} 
Let $\hat {\bm x}$ and $\hat {x _i}$ be decoded sample $Dec_{\theta}(\bm z)$ and its i-th dimensional component respectively. $\delta \bm {x}$ and $\delta {x _i}$ denote $\bm {x}-\hat {\bm x}$ and ${x _i}-\hat {x _i}$, respectively.
Then, the reconstruction losses for the Gaussian distribution and Bernoulli distribution are approximated as below.

\textbf{Gaussian distribution:} \\
Gaussian distribution is described as:
\begin{eqnarray}
\label{EQ_Gaus}
 p_{\theta}(\bm x | \bm z) 
= \prod_{i=1}^{m} \frac{1}{\sqrt{2 \pi \sigma ^2}} e^{- (x_i - \hat {x_i})^2 / 2 \sigma ^2  }
= \prod_{i=1}^{m} \frac{1}{\sqrt{2 \pi \sigma ^2}} e^{- {\delta x_i}^2 / 2 \sigma ^2  }, 
\end{eqnarray}
where $\sigma$ is a hyper parameter.
Then, the reconstruction loss is denoted as:
\begin{eqnarray}
\label{EQ_Gaus}
-\log p_{\theta}(\bm x | \bm z) 
= -\log \prod_{i=1}^{m} \frac{1}{\sqrt{2 \pi \sigma ^2}} e^{- \delta x_i^2 / 2 \sigma ^2  }
= \frac{1}{2 \sigma ^2}\sum_{i=1}^{m}{\delta x_i^2}  - \frac{m}{2} \log (2 \pi \sigma ^2).
\end{eqnarray}
The first term can be rewritten as $(1 / 2 {\sigma}^2) \ {}^t \delta {\bm x} \bm I_m  \delta {\bm x}$. Thus,  $\bm G_{\bm x} =  (1 / 2 {\sigma}^2) \ \bm I_m$ holds.  $C_{\bm x}$ is derived as the second term of the last equation in Eq.\ref{EQ_Gaus}.

%%%%%%%%%%%%%%%
\textbf{Bernoulli distribution:} \\
Bernoulli distribution is described as:
%In case $n$-dimensional Bernoulli distribution is used, the reconstruction loss, called binary cross-entropy (BCE), is denoted by
% the following cross-entropy form.
%
\begin{eqnarray}
\label{EQ_Bernoulli}
p_{\theta}(\bm x | \bm z) 
= \prod_{i=1}^{m} \hat {x_i} ^ {{x_i}} \ (1 - \hat {x_i}) ^ {(1 -  {x_i})} 
\end{eqnarray}
Then, the reconstruction loss, called binary cross-entropy (BCE), is denoted as:
\begin{eqnarray}
\label{EQ_logBernoulli}
-\log p_{\theta}(\bm x | \bm z) 
&=& -\log \prod_{i=1}^{m} \hat {x_i} ^ {{x_i}} \ (1 - \hat {x_i}) ^ {(1 -  {x_i})} 
\nonumber \\
&=& \sum_{i=1}^{m}(- x_i \log{\hat {x_i}} - (1 - x_i) \log {(1 -  {x_i})} )\nonumber \\
&=& \sum_{i}( - x_i \log (x_i + \delta x_i) -(1 - x_i ) \log(1- x_i - \delta x_i) ) \nonumber \\ 
%&=& \sum_{i}\left( - x_i \log \left(x_i \left(1 + \frac{ \Delta x_i}{x_i} \right) \right) \nonumber \\ 
%& &     - \left(1 - x_i \right) \log \left( \left(1- x_i \right) \left(1 - \frac{\Delta x_i}{1- x_i} \right) \right) \right) \nonumber \\ 
&=&  \sum_{i}\left( - x_i \log \left(1 + \frac{ \delta x_i}{x_i} \right) -\left(1 - x_i \right) \log \left(1 - \frac{\delta x_i}{1- x_i} \right) \right) \nonumber \\
& & + \sum_{i}( - x_i \log (x_i) -(1 - x_i ) \log(1- x_i) ). 
\end{eqnarray}
Here, the second term of the last equation is a constant $C_x$ depending on $\bm x$. Using Maclaurin expansion of logarithm, the first term of the last equation is further expanded as follows:
\begin{eqnarray}
\label{BCE3}
\sum_{i} \left(  - x_i \left(\frac{ \delta x_i}{x_i}   -  \frac{{\delta x_i}^2}{2 {x_i}^2} \right) 
 - \left(1 - x_i \right) \left( - \frac{\delta x_i}{1- x_i} -  \frac{{\delta x_i}^2}{2 \left(1- x_i \right)^2}\right) + O \left({\delta x_i}^3 \right) \right) \nonumber \\
= \sum_{i} \left( \frac{1}{2} \left(\frac{1}{x_i}+\frac{1}{1-x_i} \right){{\delta x_i}^2} +  O \left({\delta x_i}^3 \right) \right). 
\end{eqnarray}
Then, a metric tensor $\bm G_{\bm x}$ can be approximated as the following positive definite matrix:
%
%\begin{eqnarray}
\begin{align}\label{ax_bce}
\bm G_{\bm x} =  
  \left(
    \begin{array}{ccc}
      \frac{1}{2}\left(\frac{1}{x_1}+\frac{1}{1-x_1}\right) & 0 & \ldots \\
      0 & \frac{1}{2}\left(\frac{1}{x_2}+\frac{1}{1-x_2}\right) & \ldots \\
      \vdots & \vdots & \ddots  \\
    \end{array}
  \right). \nonumber \\
\end{align} 
%\end{eqnarray}
Here, the loss function in each dimension  $\frac{1}{2}\left(\frac{1}{x_1}+\frac{1}{1-x_1}\right)$ is a downward-convex function as shown in Figure \ref{Fig:BCEFig}. 

\begin{figure}[t]
  \begin{center}
   \includegraphics[width=70mm]{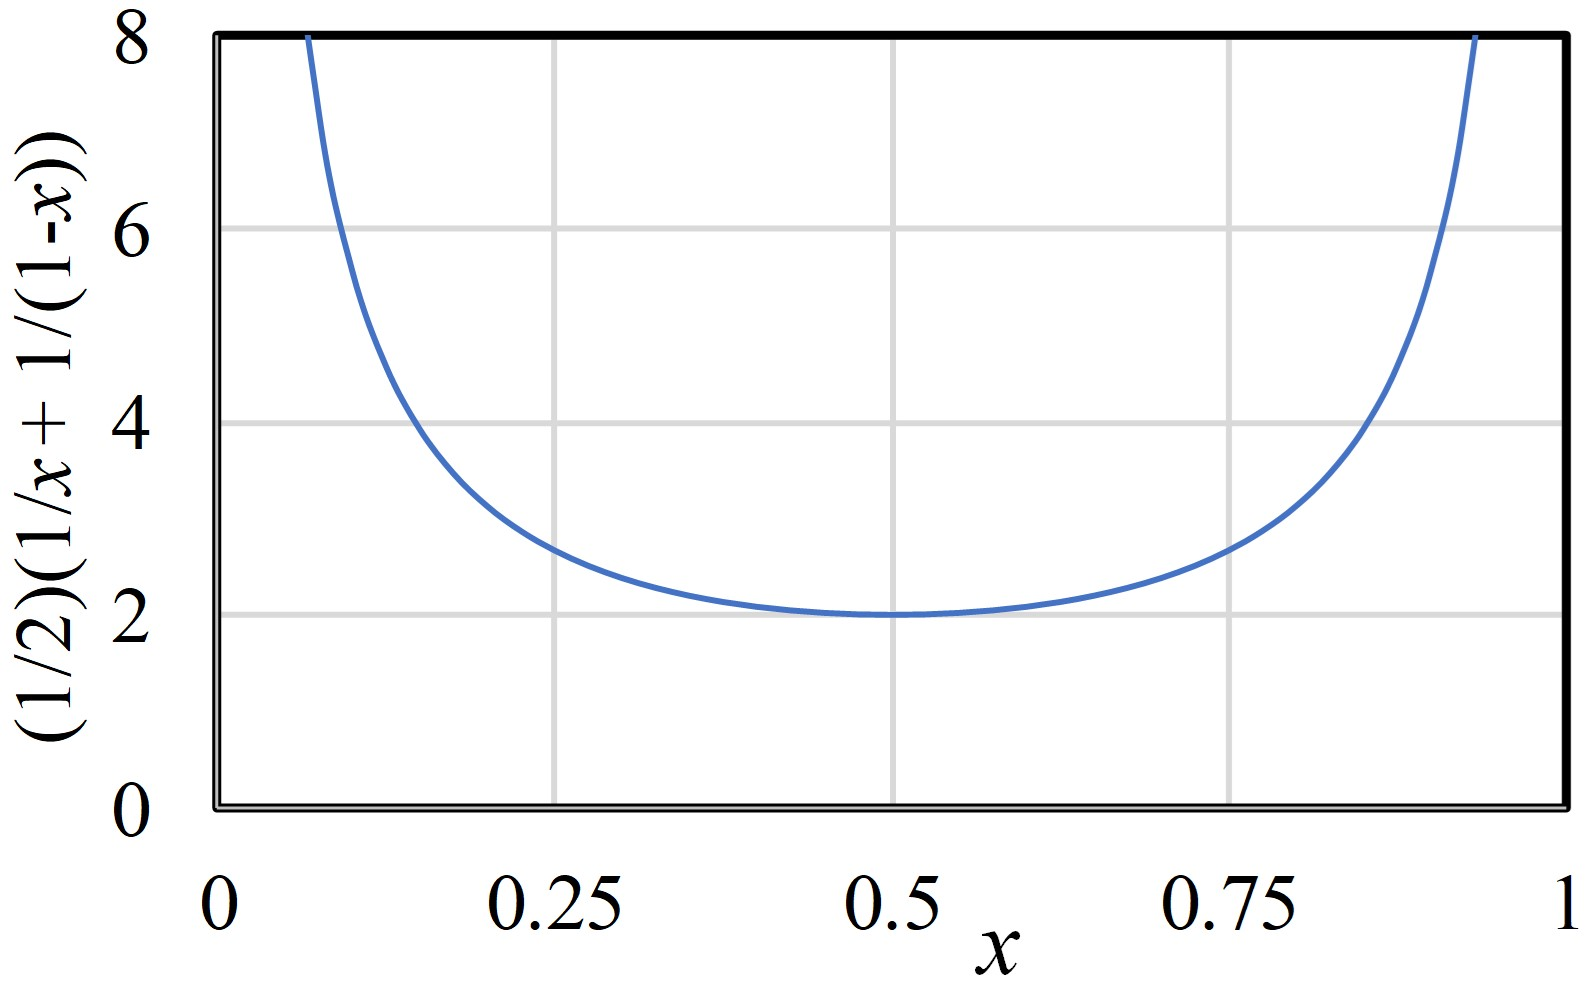}
  \end{center}
  \caption{Graph of $\frac{1}{2}\left(\frac{1}{x_1}+\frac{1}{1-x_1}\right)$.}
\label{Fig:BCEFig}
\end{figure}

%%%%%%%%%%%%%%%%%%%%%%%%%%%%%%%%%%%%%%%%%%%%%%%%%%%%%%%%%%%%%%%%%%
\subsection{Approximation of KL-divergence}
\label{sec:ApproxRateLoss}
Let $P_{z_j}$ and $R_{z_j}$ be the probability and rate to encode $z_j \sim N(0,1)$ with mean $\mu_{j({\bm x})}$ and coding noise ${\sigma_{j({\bm x})}} ^ 2$ using uniform quantization. 
Let $T$ be a quantization step with coding noise ${\sigma_{j({\bm x})}} ^ 2$, and $T = 2 \sqrt{3} {\sigma _{j({\bm x})}}$ holds from Eq.\ref{EQ_Noise}. As shown in Fig.\ref{fig:ProbAcc}, $P_{z_j}$ is denoted by $\int _{\mu_{j({\bm x})} - T/2}^{\mu_{j({\bm x})} + T/2} p(z_j) \mathrm{d}z_j$ where $p(z_j)$ is $N(0,1)$. By using Simpson's numerical integration method and $e^x = 1+x+O(x^2)$ expansion, $P_{z_j}$ is approximated by 
\begin{eqnarray}
\label{EQ_Pms}
P_{z_j} 
%\sim  {\textstyle \frac{T}{6}} \left(p ({\mu_{j({\bm x})}} - {\textstyle \frac{T}{2}} ) + 4p ({\mu_{j({\bm x})}} )+p ({\mu_{j({\bm x})}} +  {\textstyle \frac{T}{2}} ) \right) \nonumber \\
\sim  \frac{T}{6} \left(p ({\mu_{j({\bm x})}} - {\textstyle \frac{T}{2}} ) + 4p ({\mu_{j({\bm x})}} )+p ({\mu_{j({\bm x})}} +  {\textstyle \frac{T}{2}} ) \right) \nonumber \\
%&=&  \frac{T}{6 \sqrt{2 \pi}} \left(e ^{-\frac{\left({\mu} - T/2 \right)^2}{2}} + 4 e^{- \frac{ {\mu}^2}{2}}  +e ^{-\frac{\left({\mu} + T/2 \right)^2}{2}} \right) \nonumber \\
=  \frac{T p ({\mu_{j({\bm x})}}  )}{6} \biggl(4 + e ^\frac{ 4 \mu_{j({\bm x})} T  - T^2}{8}  +  e ^\frac{ -4 \mu_{j({\bm x})} T  - T^2}{8} \biggr ) \hspace{2mm} \nonumber \\
%\sim T p \left({\mu_{j({\bm x})}}  \right) \left( 1 - \frac{T^2}{24} \right) \hspace{35mm} \nonumber \\ 
\sim T p \left({\mu_{j({\bm x})}}  \right) \left( 1 - {T^2}/{24} \right) \hspace{33mm} \nonumber \\ 
= \sqrt{\frac{6}{\pi}} {\sigma_{j({\bm x})}} \ e^{ - ({\mu_{j({\bm x})}}^2)/{2}} \left( 1 - \frac{{\sigma_{j({\bm x})}}^2}{2} \right)  \hspace{15mm}
\end{eqnarray}
%\begin{equation}
%\ %Dummy
%\end{equation}
%
\if0
\begin{eqnarray}
\label{EQ_Pms}
P_{\mu\sigma} 
&\sim&  \frac{T}{6} \left(p \left({\mu} - T/2 \right) + 4p \left({\mu}  \right)+p \left({\mu} + T/2 \right) \right) \nonumber \\
%&=&  \frac{T}{6 \sqrt{2 \pi}} \left(e ^{-\frac{\left({\mu} - T/2 \right)^2}{2}} + 4 e^{- \frac{ {\mu}^2}{2}}  +e ^{-\frac{\left({\mu} + T/2 \right)^2}{2}} \right) \nonumber \\
&=&  \frac{T e^{ - \frac{{\mu}^2}{2}}}{6 \sqrt{2 \pi}} \left(4 + e ^{ \mu T /2 - T^2/8}  +  e ^{- \mu T /2 - T^2/8} \right ) \nonumber \\
&\sim& \frac{T e^{ - \frac{{\mu}^2}{2}}}{\sqrt{2 \pi}} \left( 1 - \frac{T^2}{24} \right) \nonumber \\ 
&=& \sqrt{\frac{6}{\pi}} \sigma e^{ - \frac{{\mu}^2}{2}} \left( 1 - \frac{\sigma^2}{2} \right)
\end{eqnarray}
\fi
By using $\log (1+x) = x + O(x^2)$, $R_{\mu\sigma}$ is derived by 
\begin{eqnarray}
\label{EQ_Rms}
R_{z_j} 
= -\log P_{z_j} \hspace{44mm} \nonumber \\
\sim \frac{1}{2}\left( {\mu _{j({\bm x})}}^2 + {\sigma_{j({\bm x})}} ^2 - \log {\sigma_{j({\bm x})}}^2 - \log \frac{6}{\pi} \right)
\end{eqnarray}
\if0
\begin{eqnarray}
\label{EQ_Rms}
R_{z_j} 
&=& -\log P_{z_j} \nonumber \\
&\sim& -\frac{1}{2}\left( {\mu _{j({\bm x})}}^2 + {\sigma_{j({\bm x})}} ^2 - \log {\sigma_{j({\bm x})}}^2 - \log \frac{6}{\pi} \right)
\end{eqnarray}
\fi
When Eq.\ref{EQ_DKL} and Eq.\ref{EQ_Rms} are compared, both equations are equivalent except a small constant difference $(1-\log(6/\pi))/2 \sim 0.176$ for each dimension. 
As a result, KL-divergence for j-th dimension can be considered as the rate to encode $z_j$ with mean ${\mu _{j({\bm x})}}$ and noise ${\sigma_{j({\bm x})}} ^2$.
To make theoretical analysis easier, we use the simpler approximation $P_{z_j} \sim T \ p({\mu_{j({\bm x})}}) = 2 \sqrt{3} {\sigma_{j({\bm x})}} \  p({\mu_{j({\bm x})}})$ in Fig.\ref{fig:ProbAprx} instead of Eq.\ref{EQ_Pms}.
Finally, $D_{\mathrm{KL}}(\cdot)$ is reformulated by
\if0
\begin{eqnarray}
D_{\mathrm{KL}}(\cdot)&\sim&\sum_{j=1}^{n}-\log(2 \sqrt{3} \  \sigma_{j({\bm x})} \ p(z_j)) \nonumber \\
%&=& -\log \left ( \prod _{j=1}^{n} {\sigma}_{\bm xj} \  p(z_j)\right ) -n \log (2 \sqrt{3}) \nonumber \\
&=& -\sum_{j=1}^{m} \log \left ({\sigma}_{\bm xj} \  p(z_j) \right ) -n \log (2 \sqrt{3}) \nonumber \\
&=& -\log \bigl ( p(\bm z) \prod _{j=1}^{n} {\sigma}_{\bm xj} \bigr )-n \log (2 \sqrt{3})
\end{eqnarray}
\fi
\begin{eqnarray}
\label{EQ_KLAPX}
%D_{\mathrm{KL}}(\cdot) \sim \sum_{j=1}^{m}-\log(2 \sqrt{3} \ \sigma_{j({\bm x})} \ p({\mu}_{j({\bm x})}))\hspace{19mm} \nonumber \\
D_{\mathrm{KL}}(\cdot) \sim \sum_{j=1}^{m}-\log(2 \sqrt{3} \ \sigma_{j({\bm x})} \ 
 \underset{{}^{ N(0,1)} }{\underline {p({\mu}_{j({\bm x})})}}
)\hspace{19mm} \nonumber \\
%= -\log \left ( \prod _{j=1}^{n} {\sigma}_{j({\bm x})} \  p(z_j)\right ) -n \log (2 \sqrt{3}) \hspace{2mm} \nonumber \\
%= -\sum_{j=1}^{m} \log \left ({\sigma}_{j({\bm x})} \  p({\mu}_{j({\bm x})}) \right ) -n \log (2 \sqrt{3}) \hspace{5mm} \nonumber \\
= -\sum_{j=1}^{m} \log \left ({\sigma}_{j({\bm x})} \  p({\mu}_{j({\bm x})}) \right ) -n \log (2 \sqrt{3}) \hspace{5mm} \nonumber \\
%= -\log \Bigl( p({\bm \mu}_{({\bm x})}) \prod _{j=1}^{m} {\sigma}_{j({\bm x})} \Bigr )-n \log (2 \sqrt{3}) \hspace{6mm} 
= -\log \Bigl( 
 \underset{{}^{ N_m(0,\bm I_m)} }{\underline {p(\bm \mu_{(\bm x)})}}
\prod _{j=1}^{m} {\sigma}_{j({\bm x})} \Bigr )-n \log (2 \sqrt{3}) \hspace{6mm} \end{eqnarray}
%
%%% Figure 2 %%%%%%%%%%%%%%%%%%%%%%%%%%%%%%%%%%%%%%%%%%%%%%%%%%%%%%%
%
\begin{figure}[t]
% \begin{minipage}{0.5\hsize}
 \begin{minipage}[b]{.45\linewidth}
  \begin{center}
   \includegraphics[width=50mm]{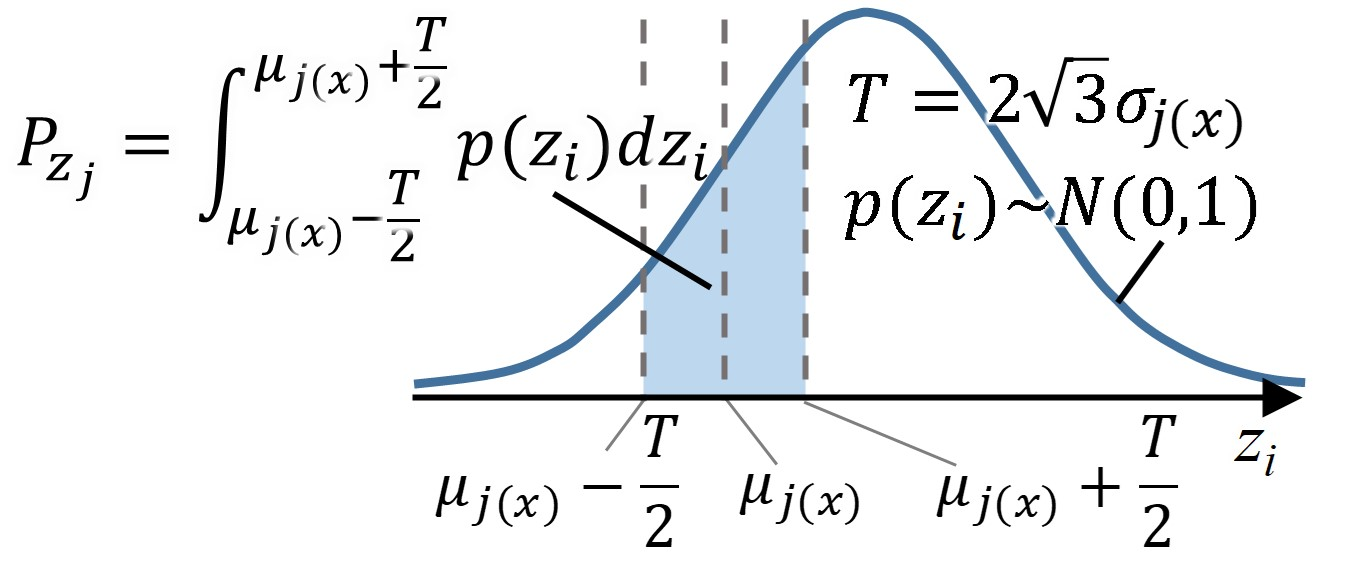}
  \end{center}
  \subcaption{Probability $P_{z_j}$}
  \label{fig:ProbAcc}
 \end{minipage}
%　
% \begin{minipage}{0.5\hsize}
 \begin{minipage}[b]{.45\linewidth}
  \begin{center}
   \includegraphics[width=50mm]{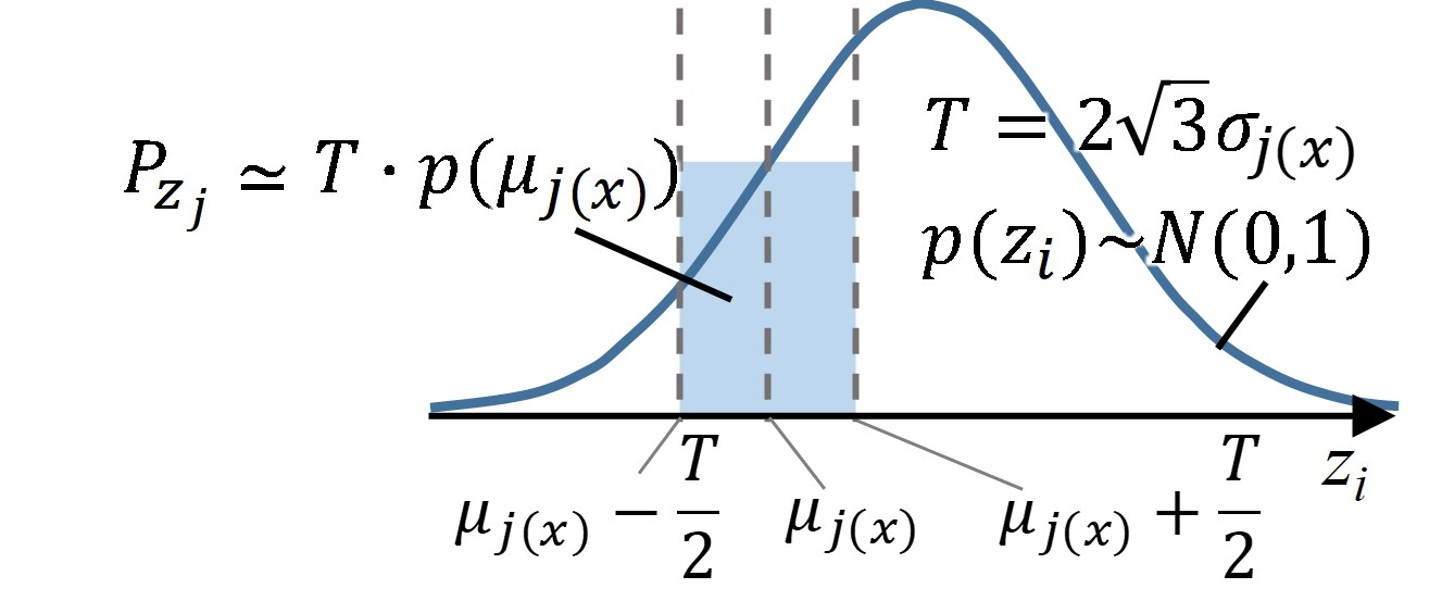}
  \end{center}
  \subcaption{Approximation of $P_{z_j}$}
  \label{fig:ProbAprx}
 \end{minipage}
%\caption{Probability $P_{\mu \sigma}$ for a symbol with mean $\mu$ and variance $\sigma^2$}
\caption{Probability for a symbol with mean $\mu$ and noise $\sigma^2$}
\label{fig:Probability}
\end{figure}
%%%%%%%%%%%%%%%%%%%%%%%%%%%%%%%%%%%%%%%%%%%%%%%%%%%%%%%%%%%%%%%%
\fi

　
%%%%%%%%%%%%%%%%%%%%%%%%%%%%%%%%%%%%%%%%%%%%%%%%%%%%%%%%%%%%%%%%
\section{Additional results in the toy dataset}
\label{AblationToy}
In this appendix, additional results for the toy dataset is explained.

\subsection{Additional coding loss}
In section \ref{ExpToyData}, two types of coding loss, square error and scaled square error (Eq.\ref{ScaledError}) are introduced.  In this subsection, we define the third coding loss in order to further evaluate the effect of nonlinearity. We define the third coding loss as follows.
\begin{eqnarray}
\label{ScaledError2}
D_2(\breve {\bm x}, \hat {\bm x}) = \frac{1}{1/2 + \|\breve {\bm x}\|_2^2 /18} \ \|\breve {\bm x}-\hat {\bm x}\|_2^2
\end{eqnarray}
We call this loss as an inversely scaled square error. In this loss, the reciprocal of the scaling factor in Eq.\ref{ScaledError} is multiplied to the square error.
Table \ref{TBLA1} shows the measurements of $ {\sigma_{j(\bm x)}}^{-2} $, $\frac{2}{\beta}{\sigma_{j(\bm x)}}^{2} D^{\prime}_j(\bm z)$, and $D^{\prime}_j(\bm z)$.  The averages of $\frac{2}{\beta}{\sigma_{j(\bm x)}}^{2} D^{\prime}_j(\bm z)$ are also close to 1 as expected, while the average of $D^{\prime}_j(\bm z)$ are different. The standard deviation values are relatively large.

The average of ${\sigma_{j(\bm x)}}^{-2}$ and its ratio are also shown in the table. Compared to Table \ref{TBL_TOY1} and \ref{TBL_TOY2}, the value of $z_3$ becomes larger.  
In the inversely scaled square error coding loss, it is assumed that the region in the data space with the larger norm is somewhat enlarged as opposed to the scaled coding loss, and the maximum variance corresponding to $ s_3 $ becomes larger.  

Figure \ref{fig:Scat1ISMSE} shows the scattering graph of data generation probabilities $p(\bm x)$ and the prior probabilities $p(\bm \mu_{(\bm x)})$ for the third coding loss. This result also shows that it is difficult to estimate data generation probability only from the prior. Correlation coefficients shown as "R" are also low.  
Next, Figure \ref{fig:Scat2ISMSE} shows the scattering graph of data generation probabilities $p(\bm x)$ and the estimated probabilities $|\bm G_{\bm x}|^{1/2} p(\bm \mu_{(\bm x)}) \prod _j \sigma _{j(\bm x)}$ for the third coding loss.
This graph also shows the proportional tendency with higher correlation coefficient 0.87, supporting the third expected property.

\begin{table}[b] 
  \caption{Measurements of toy data trained VAE using inversely scaled square error coding loss.} 
  \label{TBLA1} 
  \begin{tabular}{r|lll} 
  latent variable & $z_1$	& $z_2$	& $z_3$ \\  \hline \hline 
%#################################################### 
$\frac{2}{\beta}{\sigma_{j(\bm x)}}^{2} D^{\prime}_j(\bm z)$ \hspace{2mm} avg. & 
   0.999 & 0.953 & 1.000 \\ 
sd. & 
   0.047 & 0.183 & 0.071 \\ \hline 
%#################################################### 
$D^{\prime}_j(\bm z)$ \hspace{13mm} avg. & 
   0.266 & 1.134 & 4.710 \\ 
sd. & 
   0.103 & 0.819 & 3.423 \\ \hline 
%#################################################### 
$ {\sigma_{j(\bm x)}}^{-2} $ \hspace{11mm}	 avg. & 
   5.30e+2 & 2.28e+3 & 9.41e+3 \\ 
{\footnotesize (Ratio)}	\hspace{2mm}avg. & 
   1.000 & 4.302 & 17.753 \\ \hline 
  \end{tabular} 
\end{table} 

\begin{figure}[t]
% \begin{minipage}{0.5\hsize}
 \begin{minipage}[t]{.47\linewidth}
  \begin{center}
   \includegraphics[width=42mm]{figs/IScaled_z_plot_mix_pn_800_P(x)_vs_P(mu).png}
  \end{center}
  \subcaption{$p(\bm x)$ vs $p({\bm \mu}_{(\bm x)})$}
  \label{fig:Scat1ISMSE}
 \end{minipage}
　
% \begin{minipage}{0.5\hsize}
 \begin{minipage}[t]{.47\linewidth}
  \begin{center}
   \includegraphics[width=42mm]{figs/IScaled_z_plot_mix_pn_800_P(x)_vs_(sqrt(A)_sigma_P(mu)).png}
  \end{center}
%  \subcaption{$p(\bm x)$ vs $p({\bm \mu}_{(\bm x)})\prod_j \sigma_{(\bm x)j}$}
  \subcaption{$p(\bm x)$ vs $|\bm G|^{\frac{1}{2}}p({\bm \mu})\prod_j \sigma_{j}$}
  %  \subcaption{$(P(\bm x),P(\bm z)\prod_j \sigma_j\right)$}
  \label{fig:Scat2ISMSE}
 \end{minipage}
%\caption{Probability $P_{\mu \sigma}$ for a symbol with mean $\mu$ and variance $\sigma^2$}
\caption{Scattering plots of data generation probabilities vs. estimated probabilities for inversely scaled square error coding loss.}
\label{fig:ScatISMSE}
\end{figure}
%
%\if0
%%%%%%%%%%%%%%%%%%%%%%%%%%%%%%%%%%%%%%%%%%%%%%%%%%%%%%%%%%%%%%%%
\subsection{Consideration of a more accurate form of estimated variance for implicit orthonormal latent variables}

In section \ref{ExpObsv}, the estimated variance of the implicit orthonormal latent variables is shown as Eq.\ref{EQ_OBSV2}.
In this subsection, a more accurate form is discussed.
For given data $w$, the variance $\mathrm{Var}(w)$ is given by $E[w^2]-(E[w])^2$. In Eq.\ref{EQ_OBSV2}, the effect of the mean is ignored. To derive a more accurate form of the estimated variance, the mean of the latent variable is estimated by the following equation.
\begin{eqnarray}
\label{EQ_OBSV2_Mean}
&\ & \int {y_j} p(y_j) \mathrm{d} y_j  \nonumber \\
&\ &=  \int \left ( \frac{\mathrm{d} y_j}{\mathrm{d} z_j}{z_j} \right)  p(z_j) \mathrm{d} z_j  \nonumber \\
&\ &=\sqrt{\frac{\beta}{2}} \int \left (\frac{z_j}{{\sigma}_{j({\bm x})}} \right) p(z_j) \mathrm{d} z_j   \nonumber \\
&\ &= \sqrt{\frac{\beta}{2}} \int |{z_j}| \left (\frac{\mathrm{sign}(z_j)}{{\sigma}_{j({\bm x})}} \right) p(z_j) \mathrm{d} z_j   \nonumber \\
%&\sim&  \int {{\sigma}_{j({\bm x})}}^{-2} p(z_j) \mathrm{d} z_j \int  {z_j} ^2 p(z_j) \mathrm{d} z_j \nonumber \\
&\ &\sim \sqrt{ \frac{\beta}{2} } \int \frac{\mathrm{sign}(z_j)}{{\sigma}_{j({\bm x})}} p(z_j)  \mathrm{d} z_j \underset{=2/\sqrt{2 \pi}}{\underline {\int  |{z_j}| p(z_j) \mathrm{d} z_j}} \nonumber \\
&\ &\sim \frac{\beta}{\sqrt{\pi}} \ \ \underset{\bm x \sim p(\bm x)}{E} \left[\frac{\mathrm{sign}({\mu}_{j({\bm x})})}{{\sigma}_{j({\bm x})}} \right ]
\end{eqnarray}
Here, $\mathrm{sign}(x)$ is a sign function which returns 1 if $x>0$, returns 0 if $x=0$, and returns -1 if $x<0$.
Because the distribution of ${\mu}_{j({\bm x})}$ is close to $N(0,1)$ after training with data $\bm x$, about 50 percent of $\mathrm{sign}({\mu}_{j({\bm x})})$ is 1 and another 50 percent of $\mathrm{sign}({\mu}_{j({\bm x})})$ is -1. Therefore, Eq.\ref{EQ_OBSV2_Mean} is expected to be close to 0, and Eq.\ref{EQ_OBSV2} is still a good estimation of variance.

Using Eq.\ref{EQ_OBSV2_Mean}, more accurate form of the variance can be described by
\begin{eqnarray}
\label{EQ_OBSV2_Var}
\mathrm{Var}(y_j) 
&=& 
\frac{\beta}{2} \Biggl( \underset{\bm x \sim p(\bm x)}{E}[{{\sigma}_{j({\bm x})}}^{-2}] 
\nonumber \\
&\ & -\frac{2}{\pi} \Bigl(  \ \ \underset{\bm x \sim p(\bm x)}{E} \left[\frac{\mathrm{sign}({\mu}_{j({\bm x})})}{{\sigma}_{j({\bm x})}} \right ] \Bigr)^2 \Biggr)
\end{eqnarray}
Tables \ref{TBL11}-\ref{TBL13} show the comparison of the estimated variance using Eq.\ref{EQ_OBSV2} and Eq.\ref{EQ_OBSV2_Var} for the toy dataset.
It is observed that the difference between Eq.\ref{EQ_OBSV2} and \ref{EQ_OBSV2_Var} is relatively small.

%\begin{spacing}{1.1}
\begin{table}[H] 
  \caption{Comparison of the estimated variance of the implicit orthonormal latent variables between the simple form and accurate form for the square error coding loss. $s(\cdot)$ denotes a sign function.} 
  \label{TBL11} 
  \begin{tabular}{r|lll} 
  latent variable & $z_1$	& $z_2$	& $z_3$ \\  \hline \hline 
%#################################################### 
%$ {\sigma_{j(\bm x)}}^{-2} $ \hspace{11mm}	 avg. & 
%$ {\sigma_{j}}^{-2} $ \hspace{11mm}	 avg. & 
%${}^{\ }$ & & &\\
$ \overline{{\sigma_{j}}^{-2}} $ \hspace{22mm}	  & 
   3.87e+02 & 1.57e+03 & 6.07e+03 \\ 
%{\footnotesize (Ratio)}	\hspace{2mm}avg. & 
Ratio & 
   1.000 & 4.061 & 15.696 \\ \hline 
%#################################################### 
%$ {\sigma_{j(\bm x)}}^{-2} - mean^2$  \hspace{1mm}	 avg. & 
$ \overline{{\sigma_{j}}^{-2}} - \overline {s(\mu_{j}) \cdot {\sigma_{j}}^{-1}}^2$   & 
   3.87e+02 & 1.57e+03 & 5.73e+03 \\ 
%{\footnotesize (Ratio)}	\hspace{2mm}avg. & 
Ratio & 
   1.000 & 4.060 & 14.818 \\ \hline 
  \end{tabular} 
\end{table} 

\begin{table}[H] 
  \caption{Comparison of the estimated variance of the implicit orthonormal latent variables between the simple form and accurate form for the scaled square error coding loss. $s(\cdot)$ denotes a sign function.} 
  \label{TBL12} 
  \begin{tabular}{r|lll} 
  latent variable & $z_1$	& $z_2$	& $z_3$ \\  \hline \hline 
%#################################################### 
%$ {\sigma_{j(\bm x)}}^{-2} $ \hspace{11mm}	 avg. & 
$ \overline{{\sigma_{j}}^{-2}} $ \hspace{22mm}	  & 
   2.93e+02 & 1.17e+03 & 3.97e+03 \\ 
%{\footnotesize (Ratio)}	\hspace{2mm}avg. & 
Ratio & 
   1.000 & 3.997 & 13.536 \\ \hline 
%#################################################### 
%$ {\sigma_{j(\bm x)}}^{-2} - mean^2$  \hspace{1mm}	 avg. & 
$ \overline{{\sigma_{j}}^{-2}} - \overline {s(\mu_{j}) \cdot {\sigma_{j}}^{-1}}^2$   & 
   2.93e+02 & 1.17e+03 & 3.82e+03 \\ 
%{\footnotesize (Ratio)}	\hspace{2mm}avg. & 
Ratio & 
   1.000 & 3.997 & 13.055 \\ \hline 
  \end{tabular} 
\end{table} 

\begin{table}[H] 
  \caption{Comparison of the estimated variance of the implicit orthonormal latent variables between the simple form and accurate form for the inversely scaled square error coding loss. $s(\cdot)$ denotes a sign function.} 
  \label{TBL13} 
  \begin{tabular}{r|lll} 
  latent variable & $z_1$	& $z_2$	& $z_3$ \\  \hline \hline 
%#################################################### 
%$ {\sigma_{j(\bm x)}}^{-2} $ \hspace{11mm}	 avg. & 
$ \overline{{\sigma_{j}}^{-2}} $ \hspace{22mm}	  & 
   5.30e+02 & 2.28e+03 & 9.41e+03 \\ 
%{\footnotesize (Ratio)}	\hspace{2mm}avg. & 
Ratio & 
   1.000 & 4.302 & 17.753 \\ \hline 
%#################################################### 
%$ {\sigma_{j(\bm x)}}^{-2} - mean^2$  \hspace{1mm}	 avg. & 
$ \overline{{\sigma_{j}}^{-2}} - \overline {s(\mu_{j}) \cdot {\sigma_{j}}^{-1}}^2$   & 
   5.30e+02 & 2.28e+03 & 8.73e+03 \\ 
%{\footnotesize (Ratio)}	\hspace{2mm}avg. & 
Ratio & 
   1.000 & 4.302 & 16.462 \\ \hline 
  \end{tabular} 
\end{table} 
\if0
\begin{table}[H] 
  \caption{Comparison of the estimated variance of the implicit orthonormal latent variables between the simple form and accurate form for the inversely scaled square error coding loss. $s(\cdot)$ denotes a sign function.} 
  \label{TBL13} 
  \begin{tabular}{r|lll} 
  latent variable & $z_1$	& $z_2$	& $z_3$ \\  \hline \hline 
%#################################################### 
%$ {\sigma_{j(\bm x)}}^{-2} $ \hspace{11mm}	 avg. & 
$ \overline{{\sigma_{j}}^{-2}} $ \hspace{22mm}	  & 
   5.30e+02 & 9.41e+03 & 2.28e+03 \\ 
%{\footnotesize (Ratio)}	\hspace{2mm}avg. & 
Ratio & 
   1.000 & 17.753 & 4.302 \\ \hline 
%#################################################### 
%$ {\sigma_{j(\bm x)}}^{-2} - mean^2$  \hspace{1mm}	 avg. & 
$ \overline{{\sigma_{j}}^{-2}} - \overline {s(\mu_{j}) \cdot {\sigma_{j}}^{-1}}^2$   & 
   5.30e+02 & 8.73e+03 & 2.28e+03 \\ 
%{\footnotesize (Ratio)}	\hspace{2mm}avg. & 
Ratio & 
   1.000 & 16.462 & 4.302 \\ \hline 
  \end{tabular} 
\end{table} 
\fi
%\end{spacing}
%\fi
%
%%%%%%%%%%%%%%%%%%%%%%%%%%%%%%%%%%%%%%%%%%%%%%%%%%%%%%%%%%%%%%%%
%\subsection{Effect of $|\bm G_{\bm x}|^{\frac{1}{2}}$ to estimate the probability}
%\subsection{Effect of Gx to estimate the probability}
\subsection{Effect of $|\bm G_{\bm x}|^{\frac{1}{2}}$ to estimate the probability}
In this subsection, the effect of $|\bm G_{\bm x}|^{\frac{1}{2}}$ in Eq.\ref{EQ_OBSV3} for the probability estimation is discussed.

%First, the metric tensor $\bm G_{\bm x}$ for the square error coding loss is given by $\bm I_{m}$, as explained as the reconstruction loss for the Gaussian distribution in section \ref{ELBOAnalysis}. As a result, $|\bm G_{\bm x}|^{\frac{1}{2}}=1$ holds, which has no effect.
Because the sampling variables for a dataset generation have 3 dimensions ($s_1$, $s_2$, $s_3$), 16 dimensional toy dataset is considered to be degenerated to 3 dimensions.
Therefore, it is reasonable to consider that the metric tensor $\bm G_{\bm x}$ for the square error coding loss is a square error loss in the degenerated 3 dimensional space. As a result, $\bm G_{\bm x}$ is regarded as a $3 \times 3$ identity matrix and $|\bm G_{\bm x}|^{\frac{1}{2}}=1$ holds, which has no effect. Note that the metric tensor $\bm G_{\bm x}$ for the square coding loss is an identity matrix as explained as the reconstruction loss for the Gaussian distribution in section \ref{ELBOAnalysis}.
Next, $|\bm G_{\bm x}|^{\frac{1}{2}}$ for the scaled square error coding loss is given by $({1/2 + \|\breve {\bm x}\|_2^2 /18)})^\frac{1}{2}$.
\if0
\begin{equation}
|\bm G_{\bm x}|^{\frac{1}{2}} = ({1/2 + \|\breve {\bm x}\|_2^2 /18)})^\frac{1}{2}
\end{equation}
\fi
Third, $|\bm G_{\bm x}|^{\frac{1}{2}}$  for the inversely scaled square error coding loss is given by $({1/2 + \|\breve {\bm x}\|_2^2 /18})^{-\frac{1}{2}}$.
\if0
\begin{equation}
|\bm G_{\bm x}|^{\frac{1}{2}} = ({1/2 + \|\breve {\bm x}\|_2^2 /18})^{-\frac{1}{2}}
\end{equation}
\fi

In order to show the effect of Eq.\ref{EQ_OBSV3} for probability estimation, $p(\bm \mu_{(\bm x)}) \prod_{j=1}^{n} {{\sigma}_{j({\bm x})}}$, in which $|\bm G_{\bm x}|^{\frac{1}{2}}$ is removed from Eq.\ref{EQ_OBSV3}, is calculated  and the scattering graph  with the data generation probability $p(\bm x)$ is plotted in Figure \ref{fig:Scat3}.
%Figures \ref{fig:Scat3SMSE} and \ref{fig:Scat3ISMSE} show the scattering graphs for the scaled square error coding loss and inversely scaled square error coding loss respectively. 
%Figure \ref{fig:Scat3} shows the scattering graphs for the scaled square error coding loss and inversely scaled square error coding loss respectively. 
 In the scaled square error coding loss, the correlation coefficient according to Eq.\ref{EQ_OBSV3} is 0.8205 (Figure \ref{fig:Scat2SMSE}).  
On the other hand, the correlation coefficient without  $|\bm G_{\bm x}|^{\frac{1}{2}}$ drops to 0.6760 (Figure \ref{fig:Scat3SMSE}). 
In the inversely scaled square error coding loss, the correlation coefficient also drops from 0.8715 (Figure \ref{fig:Scat2ISMSE})  to 0.8299 (Figure \ref{fig:Scat3ISMSE}).
Therefore, these results also support  our theoretical analysis.

\begin{figure}[H]
% \begin{minipage}{0.5\hsize}
 \begin{minipage}[t]{.47\linewidth}
  \begin{center}
   \includegraphics[width=42mm]{figs/Scaled_z_plot_mix_pn_800_P(x)_vs_(sigma_P(mu)).png}
  \end{center}
  \subcaption{Scaled square error coding Loss}
  \label{fig:Scat3SMSE}
 \end{minipage}
　
% \begin{minipage}{0.5\hsize}
 \begin{minipage}[t]{.47\linewidth}
  \begin{center}
   \includegraphics[width=42mm]{figs/IScaled_z_plot_mix_pn_800_P(x)_vs_(sigma_P(mu)).png}
  \end{center}
%  \subcaption{$p(\bm x)$ vs $p({\bm \mu}_{(\bm x)})\prod_j \sigma_{(\bm x)j}$}
  \subcaption{Inversely scaled square error coding Loss}
  %  \subcaption{$(P(\bm x),P(\bm z)\prod_j \sigma_j\right)$}
  \label{fig:Scat3ISMSE}
 \end{minipage}
%\caption{Probability $P_{\mu \sigma}$ for a symbol with mean $\mu$ and variance $\sigma^2$}
\caption{Scattering plots of data generation probabilities $p(\bm x)$ vs. $p({\bm \mu})\prod_j \sigma_{j}$ where $|\bm G_{\bm x}|^{\frac{1}{2}}$ is removed from Eq.\ref{EQ_OBSV3}. Correlation coefficients are observed to be worse.}
\label{fig:Scat3}
\end{figure}

%%%%%%%
\if0
\begin{figure}[t]
  \begin{center}
   \includegraphics[width=42mm]{figs/Scaled_z_plot_mix_pn_800_P(x)_vs_(sigma_P(mu)).png}
  \end{center}
  \caption{$p(\bm x)$ vs $p({\bm \mu}_{(\bm x)})$}
  \label{fig:Scat3SMSE}
\end{figure}

\begin{figure}[t]
  \begin{center}
   \includegraphics[width=42mm]{figs/IScaled_z_plot_mix_pn_800_P(x)_vs_(sigma_P(mu)).png}
  \end{center}
  \caption{$p(\bm x)$ vs $p({\bm \mu}_{(\bm x)})$}
  \label{fig:Scat3ISMSE}
\end{figure}
\fi
\if0
%%%%%%%%%%%%%%%%%%%%%%%%%%%%%%%%%%%%%%%%%%%%%%%%%%%%%%%%%%%%%%%%
\subsection{Consideration of a more accurate form of estimated variance for implicit orthonormal latent variables}

In section \ref{ExpObsv}, the estimated variance of the implicit orthonormal latent variables is shown as Eq.\ref{EQ_OBSV2}.
In this subsection, a more accurate form is discussed.
For given data $w$, the variance $\mathrm{Var}(w)$ is given by $E[w^2]-(E[w])^2$. In Eq.\ref{EQ_OBSV2}, the effect of the mean is ignored. To derive a more accurate form of the estimated variance, the mean of the latent variable is estimated by the following equation.
\begin{eqnarray}
\label{EQ_OBSV2_Mean}
&\ & \int {y_j} p(y_j) \mathrm{d} y_j  \nonumber \\
&\ &=  \int \left ( \frac{\mathrm{d} y_j}{\mathrm{d} z_j}{z_j} \right)  p(z_j) \mathrm{d} z_j  \nonumber \\
&\ &=\sqrt{\frac{\beta}{2}} \int \left (\frac{z_j}{{\sigma}_{j({\bm x})}} \right) p(z_j) \mathrm{d} z_j   \nonumber \\
&\ &= \sqrt{\frac{\beta}{2}} \int |{z_j}| \left (\frac{\mathrm{sign}(z_j)}{{\sigma}_{j({\bm x})}} \right) p(z_j) \mathrm{d} z_j   \nonumber \\
%&\sim&  \int {{\sigma}_{j({\bm x})}}^{-2} p(z_j) \mathrm{d} z_j \int  {z_j} ^2 p(z_j) \mathrm{d} z_j \nonumber \\
&\ &\sim \sqrt{ \frac{\beta}{2} } \int \frac{\mathrm{sign}(z_j)}{{\sigma}_{j({\bm x})}} p(z_j) \mathrm{d} z_j \underset{=2/\sqrt{2 \pi}}{\underline {\int  |{z_j}| p(z_j) \mathrm{d} z_j}} \nonumber \\
&\ &\sim \frac{\beta}{\sqrt{\pi}} \ \ \underset{\bm x \sim p(\bm x)}{E} \left[\frac{\mathrm{sign}({\mu}_{j({\bm x})})}{{\sigma}_{j({\bm x})}} \right ]
\end{eqnarray}
Here, $\mathrm{sign}(x)$ is a sign function which returns 1 if $x>0$, returns 0 if $x=0$, and returns -1 if $x<0$.
Because the distribution of ${\mu}_{j({\bm x})}$ is close to $N(0,1)$ after training with data $\bm x$, about 50 percent of $\mathrm{sign}({\mu}_{j({\bm x})})$ is 1 and another 50 percent of $\mathrm{sign}({\mu}_{j({\bm x})})$ is -1. Therefore, Eq.\ref{EQ_OBSV2_Mean} is expected to be close to 0, and Eq.\ref{EQ_OBSV2} is still a good estimation of variance.

Using Eq.\ref{EQ_OBSV2_Mean}, more accrate form of the variance can be described by
\begin{eqnarray}
\label{EQ_OBSV2_Var}
\mathrm{Var}(y_j) 
&=& 
\frac{\beta}{2} \Biggl( \underset{\bm x \sim p(\bm x)}{E}[{{\sigma}_{j({\bm x})}}^{-2}] 
\nonumber \\
&\ & -\frac{2}{\pi} \Bigl(  \ \ \underset{\bm x \sim p(\bm x)}{E} \left[\frac{\mathrm{sign}({\mu}_{j({\bm x})})}{{\sigma}_{j({\bm x})}} \right ] \Bigr)^2 \Biggr)
\end{eqnarray}
Tables \ref{TBL11}-\ref{TBL13} show the comparison of the estimated variance using Eq.\ref{EQ_OBSV2} and Eq.\ref{EQ_OBSV2_Var} for the toy dataset.
It is observed that the difference between Eq.\ref{EQ_OBSV2} and \ref{EQ_OBSV2_Var} is relatively small.

%\begin{spacing}{1.1}
\begin{table}[H] 
  \caption{Comparison of the estimated variance of the implicit orthonormal latent variables between the simple form and accurate form for the square error coding loss. $s(\cdot)$ denotes a sign function.} 
  \label{TBL11} 
  \begin{tabular}{r|lll} 
  latent variable & $z_1$	& $z_2$	& $z_3$ \\  \hline \hline 
%#################################################### 
%$ {\sigma_{j(\bm x)}}^{-2} $ \hspace{11mm}	 avg. & 
%$ {\sigma_{j}}^{-2} $ \hspace{11mm}	 avg. & 
%${}^{\ }$ & & &\\
$ \overline{{\sigma_{j}}^{-2}} $ \hspace{22mm}	  & 
   3.87e+02 & 1.57e+03 & 6.07e+03 \\ 
%{\footnotesize (Ratio)}	\hspace{2mm}avg. & 
Ratio & 
   1.000 & 4.061 & 15.696 \\ \hline 
%#################################################### 
%$ {\sigma_{j(\bm x)}}^{-2} - mean^2$  \hspace{1mm}	 avg. & 
$ \overline{{\sigma_{j}}^{-2}} - \overline {s(\mu_{j}) \cdot {\sigma_{j}}^{-1}}^2$   & 
   3.87e+02 & 1.57e+03 & 5.73e+03 \\ 
%{\footnotesize (Ratio)}	\hspace{2mm}avg. & 
Ratio & 
   1.000 & 4.060 & 14.818 \\ \hline 
  \end{tabular} 
\end{table} 

\begin{table}[H] 
  \caption{Comparison of the estimated variance of the implicit orthonormal latent variables between the simple form and accurate form for the scaled square error coding loss. $s(\cdot)$ denotes a sign function.} 
  \label{TBL12} 
  \begin{tabular}{r|lll} 
  latent variable & $z_1$	& $z_2$	& $z_3$ \\  \hline \hline 
%#################################################### 
%$ {\sigma_{j(\bm x)}}^{-2} $ \hspace{11mm}	 avg. & 
$ \overline{{\sigma_{j}}^{-2}} $ \hspace{22mm}	  & 
   2.93e+02 & 1.17e+03 & 3.97e+03 \\ 
%{\footnotesize (Ratio)}	\hspace{2mm}avg. & 
Ratio & 
   1.000 & 3.997 & 13.536 \\ \hline 
%#################################################### 
%$ {\sigma_{j(\bm x)}}^{-2} - mean^2$  \hspace{1mm}	 avg. & 
$ \overline{{\sigma_{j}}^{-2}} - \overline {s(\mu_{j}) \cdot {\sigma_{j}}^{-1}}^2$   & 
   2.93e+02 & 1.17e+03 & 3.82e+03 \\ 
%{\footnotesize (Ratio)}	\hspace{2mm}avg. & 
Ratio & 
   1.000 & 3.997 & 13.055 \\ \hline 
  \end{tabular} 
\end{table} 

\begin{table}[H] 
  \caption{Comparison of the estimated variance of the implicit orthonormal latent variables between the simple form and accurate form for the inversely scaled square error coding loss. $s(\cdot)$ denotes a sign function.} 
  \label{TBL13} 
  \begin{tabular}{r|lll} 
  latent variable & $z_1$	& $z_2$	& $z_3$ \\  \hline \hline 
%#################################################### 
%$ {\sigma_{j(\bm x)}}^{-2} $ \hspace{11mm}	 avg. & 
$ \overline{{\sigma_{j}}^{-2}} $ \hspace{22mm}	  & 
   5.30e+02 & 2.28e+03 & 9.41e+03 \\ 
%{\footnotesize (Ratio)}	\hspace{2mm}avg. & 
Ratio & 
   1.000 & 4.302 & 17.753 \\ \hline 
%#################################################### 
%$ {\sigma_{j(\bm x)}}^{-2} - mean^2$  \hspace{1mm}	 avg. & 
$ \overline{{\sigma_{j}}^{-2}} - \overline {s(\mu_{j}) \cdot {\sigma_{j}}^{-1}}^2$   & 
   5.30e+02 & 2.28e+03 & 8.73e+03 \\ 
%{\footnotesize (Ratio)}	\hspace{2mm}avg. & 
Ratio & 
   1.000 & 4.302 & 16.462 \\ \hline 
  \end{tabular} 
\end{table} 
\fi
%\end{spacing}
%\subsection{Additional toy dataset}
%In
%%%%%%%%%%%%%%%%%%%%%%%%%%%%%%%%%%%%%%%%%%%%%%%%%%%%%%%%%%%%%%%%%%%%%
\subsection{Results of VAE using the conventional reconstruction loss function}

In section \ref{ExpToyData}, a decomposed loss is used for training in order to examine the effect of coding loss only.
This subsection shows that the results using a conventional reconstruction loss function form is also consistent with the theoretical analysis. 
In the experiment, the square error, which is the log-likelihood of Gaussian distribution as explained in section \ref{ELBOAnalysis}, is used as a reconstruction loss function.
%In the experiment, the square error, which is corresponding to the Gaussian distribution,  is used as a reconstruction loss function.
% which is corresponding to the Gaussian distribution as explained in section  \ref{ELBOAnalysis}.  
For training the toy data set, Eq.\ref{ToyCost2} with $\beta = 0.01$ is used as a cost function.
\begin{eqnarray}
\label{ToyCost2}
 \underset{{}^{ \bm x \sim p(\bm x) }}{E} \left[ \underset{{}^{ \bm z \sim q(\bm z|\bm x) }}{E}[{D(\bm x, \hat {\bm x})}] + \beta \ D_{KL}(\cdot)  \right ]
\end{eqnarray}

Table \ref{TBL_VAE_Conv} shows the measurements of $\frac{2}{\beta}{\sigma_{j(\bm x)}}^{2} D^{\prime}_j(\bm z)$ (Eq.\ref{EQ_OBSV1}), $D^{\prime}_j(\bm z)$, $\overline{{\sigma_{j(\bm x)}}^{-2}} $ (Eq.\ref{EQ_OBSV2}), and $ \overline{{\sigma_{j(\bm x)}}^{-2}} - \overline {\mathrm{sign}(\mu_{j(\bm x)}) \cdot {\sigma_{j(\bm  x)}}^{-1}}^2$ (Eq.\ref{EQ_OBSV2_Var}).   
As the theoretical analysis expects, $\frac{2}{\beta}{\sigma_{j(\bm x)}}^{2} D^{\prime}_j(\bm z)$ is almost close to 1. 
The ratio of the estimated variances in both Eq. \ref{EQ_OBSV2} and Eq.\ref{EQ_OBSV2_Var} is also close to the ratio of the variance of sampling variables to generate the dataset (1:4:16).

Figures \ref{fig:Scat1ConvVAE} and \ref{fig:Scat2ConvVAE} show the scattering graph of data generation probabilities $p(\bm x)$ versus  the prior probabilities $p(\bm \mu_{(\bm x)})$ and the estimated probability $|\bm G_{\bm x}|^{1/2} p(\bm \mu_{(\bm x)}) \prod _j \sigma _{j(\bm x)}$ respectively.
It can be seen that Figure \ref{fig:Scat2ConvVAE} shows the proportional property with a high correlation coefficient of 0.9003. 

As a result, these results are close to those in section \ref{ExpToyData}, which shows consistency with the theoretical analysis.
% and the results in section \ref{ExpToyData}.
%is consistent with  
%This result also shows that it is difficult to estimate data generation probability only from the prior. Correlation coefficients shown as "R" are also low.  
%Next, Figure \ref{fig:Scat2ConvVAE} shows the scattering graph of data generation probabilities $p(\bm x)$ and the estimated probabilities $|\bm G_{\bm x}|^{1/2} p(\bm \mu_{(\bm x)}) \prod _j \sigma _{j(\bm x)}$ for the third coding loss.
%This graph also shows the proportional tendency with higher correlation coefficient 0.87, supporting the third expected property.

\begin{table}[t] 
  \caption{ Measurements of toy data trained VAE using square error coding loss without loss decomposition.} 
  \label{TBL_VAE_Conv} 
  \begin{tabular}{r|lll} 
  latent variable & $z_1$	& $z_2$	& $z_3$ \\  \hline \hline 
%#################################################### 
$\frac{2}{\beta}{\sigma_{j(\bm x)}}^{2} D^{\prime}_j(\bm z)$ \hspace{2mm} avg. & 
   0.971 & 0.928 & 0.983 \\ 
sd. & 
   0.050 & 0.156 & 0.071 \\ \hline 
%#################################################### 
$D^{\prime}_j(\bm z)$ \hspace{13mm} avg. & 
   0.191 & 0.755 & 2.961 \\ 
sd. & 
   0.048 & 0.474 & 1.807 \\ \hline 
%#################################################### 
%$ {\sigma_{j(\bm x)}}^{-2} $ \hspace{11mm}	 avg. & 
$ \overline{{\sigma_{j}}^{-2}} $ \hspace{22mm}	  & 
   3.91e+01 & 1.52e+02 & 5.92e+02 \\ 
%{\footnotesize (Ratio)}	\hspace{2mm}avg. & 
Ratio & 
   1.000 & 3.896 & 15.143 \\ \hline 
%#################################################### 
%$ {\sigma_{j(\bm x)}}^{-2} - mean^2$  \hspace{1mm}	 avg. & 
$ \overline{{\sigma_{j}}^{-2}} - \overline {s(\mu_{j}) \cdot {\sigma_{j}}^{-1}}^2$   & 
   3.91e+01 & 1.52e+02 & 5.85e+02 \\ 
%{\footnotesize (Ratio)}	\hspace{2mm}avg. & 
Ratio & 
   1.000 & 3.896 & 14.951 \\ \hline 
  \end{tabular} 
\end{table} 

\begin{figure}[t]
% \begin{minipage}{0.5\hsize}
 \begin{minipage}[t]{.47\linewidth}
  \begin{center}
   \includegraphics[width=42mm]{figs/Conv_z_plot_mix2_pn_800_P(x)_vs_P(mu).png}
  \end{center}
  \subcaption{$p(\bm x)$ vs $p({\bm \mu}_{(\bm x)})$}
  \label{fig:Scat1ConvVAE}
 \end{minipage}
　
% \begin{minipage}{0.5\hsize}
 \begin{minipage}[t]{.47\linewidth}
  \begin{center}
   \includegraphics[width=42mm]{figs/Conv_plot_mix2_pn_800_P(x)_vs_(sqrt(A)_sigma_P(mu)).png}
  \end{center}
%  \subcaption{$p(\bm x)$ vs $p({\bm \mu}_{(\bm x)})\prod_j \sigma_{(\bm x)j}$}
  \subcaption{$p(\bm x)$ vs $|\bm G|^{\frac{1}{2}}p({\bm \mu})\prod_j \sigma_{j}$}
  %  \subcaption{$(P(\bm x),P(\bm z)\prod_j \sigma_j\right)$}
  \label{fig:Scat2ConvVAE}
 \end{minipage}
%\caption{Probability $P_{\mu \sigma}$ for a symbol with mean $\mu$ and variance $\sigma^2$}
\caption{Scattering plots of data generation probabilities versus estimated probabilities for square error coding loss using the conventional reconstruction loss form.}
\label{fig:ScatConvVAE}
\end{figure}

\if0
In our intuition, the ELBO cost function in the original VAE might not effectively maximize the log-likelihood.
The ELBO is derived by an approximation of log-likelihood.  Let $\mathrm{ELBO}_{\bm x}$ be a ELBO at $\bm x$. Accodingly, the probability of data $\bm x$ should be approximated by
\begin{eqnarray}
\label{EQ_ProbElbo}
P_{\theta}(\bm x) \propto \exp(\mathrm{ELBO}_{\bm x})
\end{eqnarray}

We evaluate the estimated probabilities by using both Eq.\ref{EQ_ProbElbo} and Eq.\ref{EQ_OBSV2} in the toy dataset. $\mathrm{ELBO}_{\bm x}$ in the original VAE is rewritten as
\begin{eqnarray}
\label{ToyCost2}
\mathrm{ELBO}_{\bm x} 
&=&
 - \beta^{-1}\underset{{}^{ \bm z \sim q(\bm z|\bm x) }}{E}[{D(\bm x, \hat {\bm x})}] - D_{KL}(\cdot) \nonumber \\
&\sim&
 - \frac{\beta}{2}^{-1}\bigl( D \left ( \bm x, Dec_\theta(\mu _{j(\bm x)}-\sigma_{j(\bm x)})\right) \nonumber \\
&\ & + D \left (\bm x, Dec_\theta(\mu _{j(\bm x)}+\sigma_{j(\bm x)}) \right )\bigr) \nonumber \\
&\ &  - D_{KL}(\cdot)
\end{eqnarray}

Figure shows the correlation coefficients between the data generation probability and the estimated probabilities derived by both Eq.\ref{EQ_ProbElbo} and Eq.\ref{EQ_OBSV2}.
\fi
